# Supplementary material for: Controlling spin-orbit interactions in silicon quantum dots using magnetic field direction
Source: arXiv:1807.10415 ancillary file (2019-02-15)
Supplement: Supplementary file 1 [file Supplementary_spin_orbit.pdf]

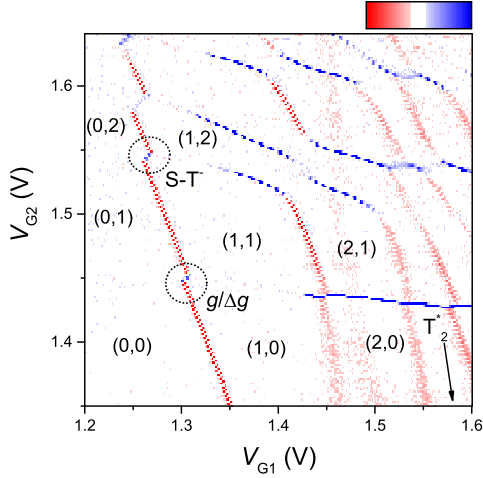

FIG. S1. Stability map of the device used here. The major operation voltages areas are encircled. The  $T_2^*$  experiment was performed around the  $V_{G1} = 1.6424$  V  $V_{G2} = 1.1760$  V operating point, outside the range of this stability map.

## I. STABILITY MAP AND OPERATION POINTS

Stability map of the device is shown in Fig. S1. There are a number of operating regions where data is collected, including: the  $g$ -tensors near the (1,0)-(0,1) anti-crossing, S- $T^-$  data near the (0,2)-(1,1) anti-crossing, and Stark shift and coherence time at the (3,0) charge state as indicated in the stability map.

## II. EXTRACTING $g$ -TENSOR

To obtain the  $g$ -tensor we use the equation

$$g^2(\varphi_B, \theta_B) = \hat{r}(\varphi_B, \theta_B)^\dagger \hat{g}_1^\dagger \hat{g}_1 \hat{r}(\varphi_B, \theta_B), \quad (1)$$

where

$$\hat{r}(\varphi_B, \theta_B)^\dagger = (\cos(\varphi_B) \cos(\theta_B), \sin(\varphi_B) \cos(\theta_B), \sin(\theta_B)) \quad (2)$$

is a unit vector pointing along the magnetic field direction. Using the measurements, we obtain the  $g$ -tensor with a least square sum fit. Furthermore, we use this tensor to estimate the  $g$ -factor in the whole  $(\varphi_B, \theta_B)$  plane. The best fit of the  $g$ -factor is presented in Fig. S2a. The dashed lines indicate at which points the data was acquired with magnetic field direction sweeps.

## III. $g$ -FACTOR DIFFERENCE OF QD1 AND QD2 AND $g$ -TENSOR OF QD2

The  $g$ -factor difference measurements can also be used to extract  $\hat{g}_2$ . We do this by using the information from the  $g$ -factor difference of QD1 and QD2 that

gives us  $\Delta g_{12}$  which we use to estimate  $g_2(\varphi_B, \theta_B) = \Delta g_{12}(\varphi_B, \theta_B) + g_{1,\text{est}}(\varphi_B, \theta_B)$ , where  $g_{1,\text{est}}(\varphi_B, \theta_B) = \sqrt{B^\dagger \hat{g}_1^\dagger \hat{g}_1 B} / |B|$ . We obtain

$$\hat{g}_2 = 1.9 \times I + \begin{pmatrix} 36.0 & -16.4 & -5.8 \\ -16.4 & 36.0 & -0.3 \\ -5.8 & -0.3 & 28.0 \end{pmatrix} \times 10^{-3}, \quad (3)$$

with 95% confidence error bar of  $\pm 10^{-3}$  for each terms, which resembles closely  $\hat{g}_1$ . This is used to estimate the difference of the  $g$ -factors presented in Fig. S2b. Similarly, as in the main text, we get the Rashba and Dresselhaus interaction strengths for the second dot to be  $\alpha_g^* = 7.32 \pm 3.96$  MHz/T and  $\beta_g^* = 119.9 \pm 7.0$  MHz/T. In addition similarly as in the main text it is unlikely that we have the an interface step in the vicinity of this dot [1–3].

In addition to the experiments presented in the main text, we measure the  $g$ -factor difference as function of in-plane magnetic field in the (1,1) charge configuration with ESR and S- $T$  latched readout. This is similar to the ESR singlet-triplet experiment that was performed earlier [4]. The pulse sequence used in this measurement is presented in Fig. S3a. First, we initialize the singlet state in (2,0). Then we pulse to (1,1) where the singlet state transfers to  $|\uparrow\downarrow\rangle$  or  $|\downarrow\uparrow\rangle$  depending on the magnetic field angle. We then use an ESR pulse to flip the spin of the other dot and readout at the latching point where the states  $|\uparrow\uparrow\rangle$  and  $|\downarrow\downarrow\rangle$  are blockaded. After readout we re-initialize in the (1,2) region. The schematic energy diagram of this anti-crossing is presented in the inset of Fig. S3a. As function of  $f_{\text{ESR}}$  we observe two peaks, where the triplet probability is increased (data not shown). We probe these two ESR frequencies as a function in-plane magnetic field angle  $\varphi_B$ . The difference of the two resonant frequencies correspond to the  $g$ -factor difference of the two dots. The results for this measurement are presented in Fig. S3b. This measurement of the absolute value of  $g$ -factor differences is very similar to the one presented earlier in a similar system [5]. We use the fit

$$\frac{\mu_B \Delta g}{h} = B(\Delta\alpha + \Delta\beta \sin(\varphi_B)), \quad (4)$$

where  $\Delta\alpha$  is the Rashba term difference,  $\Delta\beta$  is the Dresselhaus term difference of the two dots and  $h$  is the Planck constant. We extract  $|\Delta\alpha| = 2.4$  MHz/T and  $|\Delta\beta| = 24.9$  MHz/T at this operation regime.

## IV. STARK SHIFT MEASUREMENTS

The Stark shift measurements in the main text were performed by probing  $f_{\text{ESR}}$  as a function of load level depth in G1 dot. A linear fit is done to determine the shift of  $f_{\text{ESR}}$  due to the top gate voltage. The extreme values differ a lot from the one presented in (3,0) since the spin-orbit interaction strength is different. This difference in

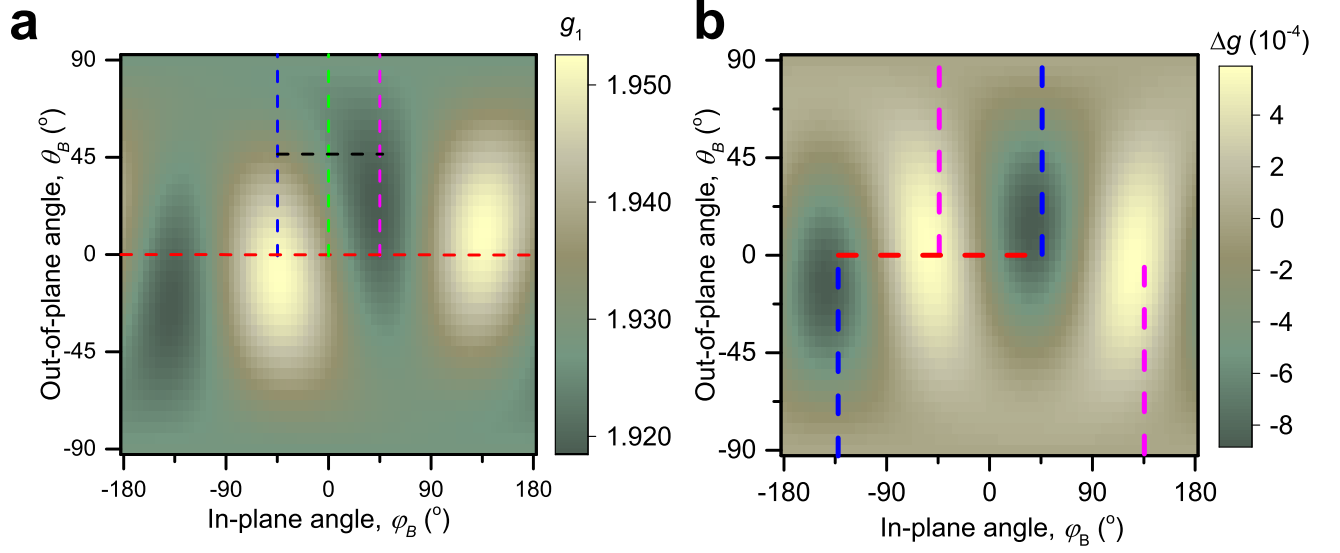

FIG. S2. Estimated  $g$ -factor and the  $g$ -factor difference between the dots. (a)  $g$ -factor of the G1 dot as a function of magnetic field angles. (b)  $g$ -factor difference of the G1 and G2 dots as a function of magnetic field angles. Isosurfaces corresponding to these graphs are presented in the main text.

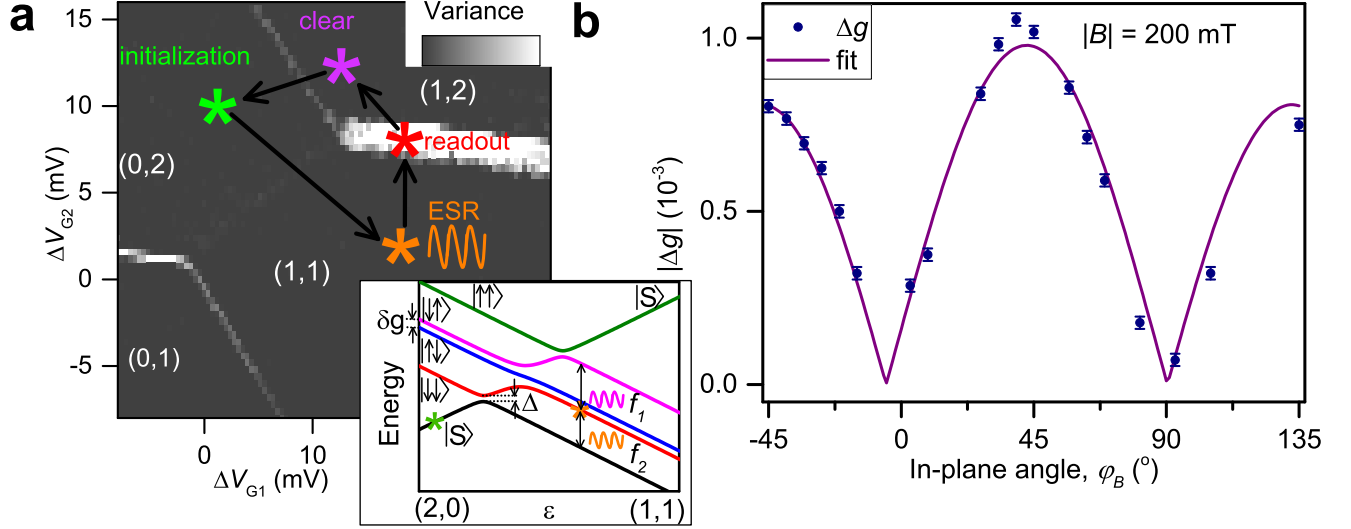

FIG. S3.  $g$ -factor difference in (1,1) region. (a) Pulse sequence used to measure  $g$ -factor difference. Inset: Energy diagram of the system near the anti-crossing. (b) Absolute value of  $g$ -factor difference as a function of in-plane magnetic field angle.

the Stark shift has been studied before and is consistent with the theories and experiments that show that the SOI strength can be significantly different between the valley states [1, 3].

To extract the Rashba coefficient in the main text from the measurements of derivative of the Stark shift, . The fit  $A \sin(2\varphi_B) + B$  vanishes at the angle  $\varphi_0 = \frac{1}{2} \arcsin(\frac{B}{A})$ . We use the notation from Ref. [2] (Eq. 50) where the angle where the derivative of the Stark shift vanishes can

be expressed as

$$\varphi_{v_i} = \frac{1}{2} \arcsin\left(\frac{\alpha_i}{\beta_i}\right). \quad (5)$$

Hence the ratio  $\alpha/\beta$  equals  $B/A$  and we can use the fits and Dresselhaus to obtain Rashba strength.

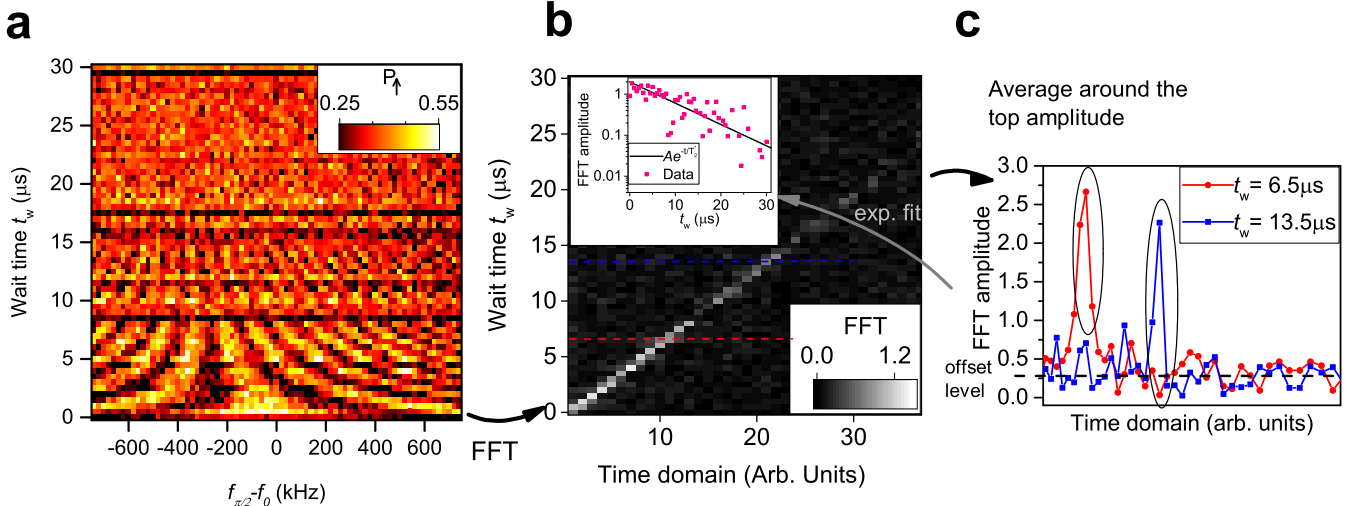

FIG. S4. Determination of  $T_2^*$  from the Ramsey measurement. (a) Example of a Ramsey interferometry experiment at  $\varphi_B = -10^\circ$ . (b) Discrete Fourier transform of (a) along the frequency axis. Inset: Amplitudes of the Fourier transform together with the fit. (c) Examples of two different line traces in (b).

## V. $T_2^*$ MEASUREMENTS

Our coherence time measurements are based on Ramsey interferometry experiments, done for each point by driving two  $\pi_x/2$  pulses and sweeping the pulse frequency around the ESR resonance and stepping the time interval between the pulses presented in Fig. S4a. To extract the  $T_2^*$  we Fourier transform each frequency sweep, which yields the amplitudes of the oscillations presented in Fig. S4b. To obtain the amplitude of the oscillations, we average three points around the expected oscillation frequency as shown in Fig. S4c. We normalize these amplitudes by subtracting the background amplitude noise level. These oscillations can be fit to a exponential decay with constant amplitude  $A_0$ . An example of such a fit is presented in the inset of Fig. S4b.

## VI. SINGLET-TRIPLET MIXING

As mentioned in the main text, there are three different mechanisms that we consider as a main suspect for the S-T<sup>-</sup> mixing  $\Delta_{S-T^-}$ . These mechanisms are hyperfine,  $g$ -factor difference, and tunneling induced SOI effects, as schematically depicted in Fig. S5c. Due to the difference between the off-diagonal terms in the  $g$ -tensors of the two dots the singlet and triplet T<sup>-</sup> states are mixed. For a moving electron, spin-orbit interaction can induce a net effective spin-orbit field [6–8]. Depending how this spin-orbit field is aligned with respect to the external magnetic field, it can cause the quantization axis to tilt slightly during tunneling yielding a finite mixing between the up and down states of the moving electron. In the main text we exclude the Overhauser field due to the residual  $^{29}\text{Si}$ .

Here we derive the expressions for both of these mixing terms and show their behaviour.

In order to obtain  $\Delta_{S\Delta g}(\varphi_B, \theta_B)$ , we renormalize the  $g$ -tensor so that it is aligned with the  $B$ -field direction. We construct an orthonormal matrix  $U$  using Gram-Schmidt for which

$$\bar{B} = U(0, 0, 1)^\dagger T. \quad (6)$$

Now the  $g$ -tensor in this new basis reads as  $\hat{g}_i^* = U^T \hat{g}_1 U$ . The mixing  $\Delta_{S\Delta g}$  can be obtained now from the matrix elements  $g_i^{zx*}$  and  $g_i^{zy*}$ . Now the difference term is  $\delta g^{zi} = \frac{g_1^{zi*} - g_i^{zi*}}{2}$ . It is worth noting that the matrix  $U$  is not unique but depends on the choice of the  $x$  and  $y$  axis in the new coordinate system. However, this choice will only change the phase of  $\Delta_{S\Delta g}$  and not the absolute value.

In Fig. S5a we show the numerically estimated square for the S-T<sup>-</sup> mixing as a function of in-plane and out-of-plane angles. This plot is obtained by using the  $g$ -tensors from the experiment. As one can see from the plot the maximum coupling is around 500 kHz, well below the observed value of 27.5 MHz. As seen in the previous section, the  $g$ -factor difference might change upon choosing different operating points the  $g$ -tensors were obtained at a different operation points, however we would not expect significantly increased mixing in this configuration.

Electron relaxation due to the SOI for a moving electron in a double dot system has been studied previously theoretically [6, 7] and experimentally [9, 10]. The moving electron induces a spin-orbit field. If this field is not aligned with the external magnetic field the quantization axis gets tilted mixing up and down states and alternatively S and T<sup>-</sup> states. First we consider the spin Hamiltonian as  $H_i = g\mu_B \bar{B} \cdot \hat{S}$ , where  $\hat{S} = (\sigma_x, \sigma_y, \sigma_z)^\dagger$ . We

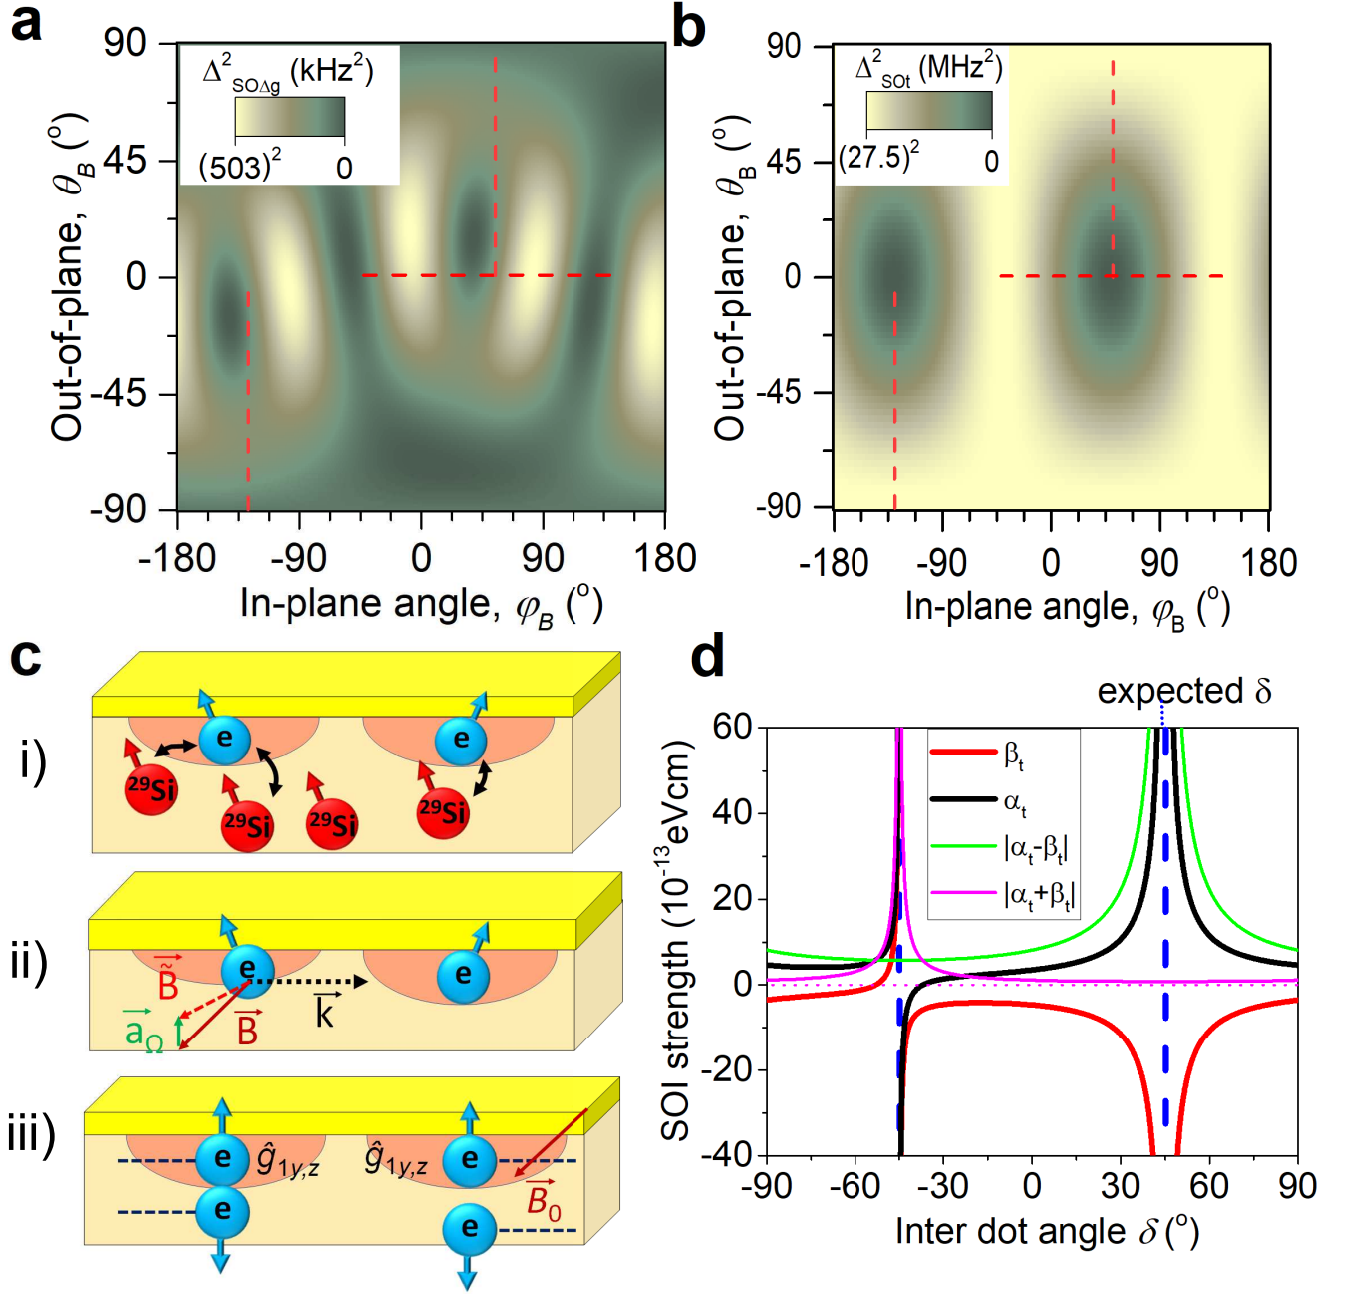

FIG. S5. Singlet-Triplet spin-flipping term origin. (a) The square of the singlet-triplet spin-flipping term as a function of magnetic field direction angles based on the estimated g-factor difference. (b) The square of the singlet-triplet splitting as a function of magnetic field direction angles based on the estimated the momentum term during the tunnelling process. Red lines in both (a) and (b) correspond to the directions along which the data was taken in Fig. 4 of the main text. (c) Schematic illustration of the possible causation of the S-T- energy splitting mechanisms. From top to bottom: i) Hyperfine interaction with residual  $^{29}\text{Si}$  nuclei. ii) spin-orbit interaction induced by moving electron. iii) spin-orbit interaction due g factor difference of the dots. d) Fitted Rashba and Dresselhaus coefficients as a function of angle for the line of dots.

can diagonalize the spin Hamiltonian in the case of fixed external magnetic field to obtain the spin eigenstates

$$|\uparrow\rangle = \begin{pmatrix} \cos(\theta'_B) \\ e^{i\varphi_B} \sin(\theta'_B) \end{pmatrix}, |\downarrow\rangle = \begin{pmatrix} -e^{i\varphi_B} \sin(\theta'_B) \\ \cos(\theta'_B) \end{pmatrix}, \quad (7)$$

where  $\theta'_B = (\theta_B - 90)/2$ .

Here, we only consider situation where only the lowest energy valley eigenstate is relevant. The  $S(0, 2)$  and  $T^-(1, 1)$  wave functions in a double dot system can be

written as

$$|T^-(1, 1)\rangle = \frac{1}{\sqrt{2}}|L_1R_2 - R_1L_2\rangle|\downarrow_1\downarrow_2\rangle \quad (8)$$

$$|S(0, 2)\rangle = \frac{1}{\sqrt{2}}|R_1R_2\rangle|\uparrow_1\downarrow_2 - \downarrow_1\uparrow_2\rangle, \quad (9)$$

where  $L_i$  and  $R_i$  correspond to the wave functions of the electrons in the Left and Right dots respectively.

We now compute the spin-orbit coupling matrix element between  $|S(0, 2)\rangle$  and  $|T^-(1, 1)\rangle$  using the spin-orbit Hamiltonian (Eq. 1 in the main text),

$$\begin{aligned} \Delta_{\text{SOt}} &= \langle S | H_{\text{SO}} | T^- \rangle \\ &= \frac{1}{2} \langle \uparrow_1\downarrow_2 - \downarrow_1\uparrow_2 | \langle R_1R_2 | H_{\text{SO}} | L_1R_2 - R_1L_2 \rangle | \downarrow_1\downarrow_2 \rangle \\ &= \frac{1}{\sqrt{2}} \langle \uparrow_1\downarrow_2 - \downarrow_1\uparrow_2 | \langle R | \alpha(k_x\sigma_y - k_y\sigma_x) \\ &\quad + \beta(k_x\sigma_x - k_y\sigma_y) | L \rangle | \downarrow_1\downarrow_2 \rangle. \end{aligned} \quad (10)$$

Now we rewrite  $\langle R | k_x | L \rangle = \langle k_\xi \rangle \cos \delta$  and  $\langle R | k_y | L \rangle = \langle k_\xi \rangle \sin \delta$ , where  $\langle k_\xi \rangle = \langle R | k_\xi | L \rangle$  is the expectation value of the electron wave operator along the line of dots. By substituting these to the equation above we get

$$\begin{aligned} \Delta_{\text{SOt}} &= \frac{1}{\sqrt{2}} \langle \uparrow_1\downarrow_2 - \downarrow_1\uparrow_2 | \langle k_\xi \rangle \alpha (\sigma_y \cos \delta - \sigma_x \sin \delta) \\ &\quad + \beta (\sigma_x \cos \delta - \sigma_y \sin \delta) | \downarrow_1\downarrow_2 \rangle \end{aligned} \quad (12)$$

$$\begin{aligned} &= \frac{\langle k_\xi \rangle}{\sqrt{2}} \langle \uparrow_1\downarrow_2 - \downarrow_1\uparrow_2 | (\alpha \cos \delta - \beta \sin \delta) \sigma_y + \\ &\quad (\alpha \sin \delta + \beta \cos \delta) \sigma_x | \downarrow_1\downarrow_2 \rangle \end{aligned} \quad (13)$$

$$\begin{aligned} &= \langle k_\xi \rangle \langle \uparrow | (\alpha \cos \delta - \beta \sin \delta) \sigma_y + \\ &\quad (\alpha \sin \delta + \beta \cos \delta) \sigma_x | \downarrow \rangle. \end{aligned} \quad (14)$$

As discussed in the main text in this case we use the  $\alpha$  and  $\beta$  that are associated with  $\frac{d}{dx}$  term and thus replace them with  $\alpha_t$  and  $\beta_t$  respectively. Hence the equation

above yields the square of the mixing term as

$$\begin{aligned} |\Delta_{\text{SOt}}|^2 &= \langle k_\xi \rangle^2 |\alpha_t \cos(\varphi_B^-) + \beta_t \sin(\varphi_B^+) \\ &\quad + i \cos(2\theta_B') (\beta_t \cos(\varphi_B^+) - \alpha_t \sin(\varphi_B^-))|^2, \end{aligned} \quad (15)$$

where  $\varphi_B^\pm = \varphi_B \pm \delta$ . Now  $\langle k_\xi \rangle$  is dependent on the exact shape of the potential well of the double dot system. Here, we assume a double parabolic well in which case this expectation value has been shown [6, 11] to equal  $\langle k_\xi \rangle = \frac{4lm_{\text{eff}}}{3\hbar}$ .

We show the fit for the normalized square of the S-T<sup>-</sup> mixing as function magnetic field direction in Fig. S5b. Here, we have chosen  $\alpha_t$ ,  $\beta_t$  and  $\delta$  such that the angular dependence is the same as in experiments. As discussed earlier in the text, we have three free parameters in the model that have an effect on two different model values: in-plane angle where the mixing vanishes and the maximum amplitude of the mixing. Hence we cannot get unique Rahba and Dresselhaus strengths by fitting the data to our model unless we assume a certain  $\delta$ . In Fig. S5d we plot  $\alpha_t$  and  $\beta_t$  together with the sum and subtraction of the them as a function of a fixed  $\delta$  fitted with the experimental data. Here, we have assumed the interdot length to equal 40 nm and the tunnel coupling to equal 6 GHz that we extracted from the spin-funnel experiment.

We note that in Fig. S5d there are two divergences at  $\delta = 45^\circ$  and  $\delta = -45^\circ$  which is arising from the model. To fit the model we assume two things: the value of  $\delta$  (that we vary) and Eq. 15. At these divergences one of the assumptions, essentially the value of  $\delta$ , is wrong. Hence the real  $\delta$  cannot equal exactly those values. From another perspective: if  $\delta = 45^\circ$  or  $\delta = -45^\circ$  there will be no  $\alpha_t$  and  $\beta_t$  that can explain the data. The minimum mixing would in those cases always be at  $\varphi_B = 45^\circ$  or  $\varphi_B = 45^\circ$  where as we observe the minimum at  $\varphi_B = 51^\circ$ . From the lithography we would assume  $\delta = 45^\circ$  which is at the point where the assumption fails. Due to the strain it is possible that the dots are not induced directly at the intended spot and might not be aligned with the gates [12] which would enough to explain the data.

- 
- [1] R. Ferdous, K. W. Chan, M. Veldhorst, J. C. C. Hwang, C. H. Yang, H. Sahasrabudhe, G. Klimeck, A. Morello, A. S. Dzurak, and R. Rahman, Phys. Rev. B **97**, 241401 (2018).
  - [2] R. Ruskov, M. Veldhorst, A. S. Dzurak, and C. Tahan, Phys. Rev. B **98**, 245424 (2018).
  - [3] M. Veldhorst, R. Ruskov, C. H. Yang, J. C. C. Hwang, F. E. Hudson, M. E. Flatté, C. Tahan, K. M. Itoh, A. Morello, and A. S. Dzurak, Phys. Rev. B **92**, 201401 (2015).
  - [4] M. A. Fogarty, K. W. Chan, B. Hensen, W. Huang, T. Tanttu, C. H. Yang, A. Laucht, M. Veldhorst, F. E. Hudson, K. M. Itoh, D. Culcer, T. D. Ladd, A. Morello, and A. S. Dzurak, Nature Communications **9**, 4370 (2018).

- [5] R. M. Jock, N. T. Jacobson, P. Harvey-Collard, A. M. Mounce, V. Srinivasa, D. R. Ward, J. Anderson, R. Manginell, J. R. Wendt, M. Rudolph, T. Pluym, J. K. Gamble, A. D. Baczewski, W. M. Witzel, and M. S. Carroll, Nat. Commun. **9**, 1768 (2018).
- [6] D. Stepanenko, N. E. Bonesteel, D. P. DiVincenzo, G. Burkard, and D. Loss, Phys. Rev. B **68**, 115306 (2003).
- [7] D. Stepanenko, M. Rudner, B. I. Halperin, and D. Loss, Phys. Rev. B **85**, 075416 (2012).
- [8] G. Burkard and D. Loss, Phys. Rev. Lett. **88**, 047903 (2002).
- [9] A. Hofmann, V. F. Maisi, T. Krähenmann, C. Reichl, (2018).

- W. Wegscheider, K. Ensslin, and T. Ihn, Phys. Rev. Lett. **119**, 176807 (2017).
- [10] P. Scarlino, E. Kawakami, P. Stano, M. Shafiei, C. Reichl, W. Wegscheider, and L. M. K. Vandersypen, Phys. Rev. Lett. **113**, 256802 (2014).
- [11] G. Burkard, D. Loss, and D. P. DiVincenzo, Phys. Rev. B **59**, 2070 (1999).
- [12] J. J. Pla, A. Bienfait, G. Pica, J. Mansir, F. A. Mohiyaddin, Z. Zeng, Y. M. Niquet, A. Morello, T. Schenkel, J. J. L. Morton, and P. Bertet, Phys. Rev. Appl. **9**, 044014 (2018).
